# Supplementary material for: Procedural Text Mining with Large Language Models
Source: arXiv:2310.03376 source file (2023-10-05)
Supplement: Supplementary file 1 [file appendix.tex]

\appendix

\section{Photography}

Format Memory Card: raw setting ChatGPT conversation \url{https://chat.openai.com/share/40cff5a0-80b6-4d51-8864-34f70ec1770e}, and ontology setting ChatGPT conversation \url{https://chat.openai.com/share/437e9bb7-66cb-4dbd-a20c-7a8e584b8d1d}

Fully Automatic Shooting: raw setting ChatGPT conversation \url{https://chat.openai.com/share/a514a64d-1b35-4017-8d80-d6209089a155}, and ontology setting ChatGPT conversation \url{https://chat.openai.com/share/5dcbb0fd-2729-49b2-8960-4812a86a3dd1}

Registering the Picture Style: raw setting ChatGPT conversation \url{https://chat.openai.com/share/945e6414-7c40-4be6-a709-c063f6d953ed}, and ontology setting ChatGPT conversation \url{https://chat.openai.com/share/ab791ae8-d27e-42ea-be9b-7db1d4fca10c}

2-shot experiments raw setting ChatGPT conversation \url{https://chat.openai.com/share/31ced131-06fc-48ba-8099-d0164d0cf6c4}

2-shot experiments ontology ChatGPT conversation \url{https://chat.openai.com/share/f4a48d1b-d716-40fe-bde1-ef1b90e556f9}

\section{Medicine}

2-Cylinder Portable System Assembly: raw setting \url{https://chat.openai.com/share/5e00f740-d180-4a8f-ace2-d32c144ba024}; ontology setting \url{https://chat.openai.com/share/2ba5112e-f831-47bf-b1c1-c64e5ba8992f}

Changing Gas Cylinders: raw setting \url{https://chat.openai.com/share/14e012c9-3975-473c-a756-a805249a5471}; ontology setting \url{https://chat.openai.com/share/e5ff9fb1-a0c7-4955-a3d2-0b8d3d367df2}

Installation of FM Type: raw setting \url{https://chat.openai.com/share/f219a3cf-6504-403a-8846-944f7ca4f762}; ontology setting \url{https://chat.openai.com/share/2585a60e-1e91-4b13-9829-439996c39911}

2-shot experiments raw setting: \url{https://chat.openai.com/share/2523069a-a243-4e83-bae3-b89fdf2f7e4b}; \url{https://chat.openai.com/share/df2e9bb1-e70d-4a05-b5a1-0138f9e9b183}

\section{Manufacturing}

Inspect the pump procedure: raw setting \url{https://chat.openai.com/share/37af6816-ddb5-436e-85ad-a1d490c4c508}; ontology \url{https://chat.openai.com/share/ba095430-a52f-4d49-9464-57f628f5aa78}

Support plate installation procedure: raw setting \url{https://chat.openai.com/share/e11a1518-f3fc-449e-a656-cb178af2be1a}; ontology \url{https://chat.openai.com/share/70a647f5-a983-4148-a57c-73e99f200d71}

Removal and installation of Mechanical seal procedure: raw setting \url{https://chat.openai.com/share/c3f36faa-4293-44a1-815f-7594f9752926}; ontology \url{https://chat.openai.com/share/c2aeb0d7-89fa-4f37-bf30-ae97b7bd6244}

2-shot experiments raw setting: \url{https://chat.openai.com/share/45549f57-82cc-4c53-9ae9-cf8bcb0cd833}; \url{https://chat.openai.com/share/242ba5d8-8b9e-4e41-8ed5-a9871ac2292d}

\section{Agriculture}

Operating the Hydrostatic Transmission procedure: raw setting \url{https://chat.openai.com/share/d837262a-5fa2-4236-ad3d-6bc872286bcc}; ontology \url{https://chat.openai.com/share/ce01a57c-aeba-4dfb-963d-1220541f4cae}

Lowering ROPS Crossbar procedure: raw setting \url{https://chat.openai.com/share/e94619c4-afe3-439c-a7a3-5e3206ca4dc6}; ontology \url{https://chat.openai.com/share/3c770be1-b3b5-4bfd-8170-9156df6bed96}

Changing Front Axle Oil procedure: raw setting \url{https://chat.openai.com/share/6f02eb22-f798-419b-91f2-635521ad559d}; ontology \url{https://chat.openai.com/share/d90b693c-b84d-48b2-8634-bbc9d6e357a7}

2-shot experiments raw setting: \url{https://chat.openai.com/share/a46f197c-77d0-40dc-8b41-28b62396eff3}; ontology \url{https://chat.openai.com/share/3391ef44-c986-45c0-bc95-fc848a6c12ab}

%%
%% End of file `sample-sigplan.tex'.
